# Supplementary material for: Leveraging Public Data for Practical Private Query Release
Source: arXiv:2102.08598 source file (2021-06-11)
Supplement: Supplementary file 1 [file compare_benchmarks_appendix.tex]

\begin{figure}%
    \centering
    \includegraphics[width=\linewidth]{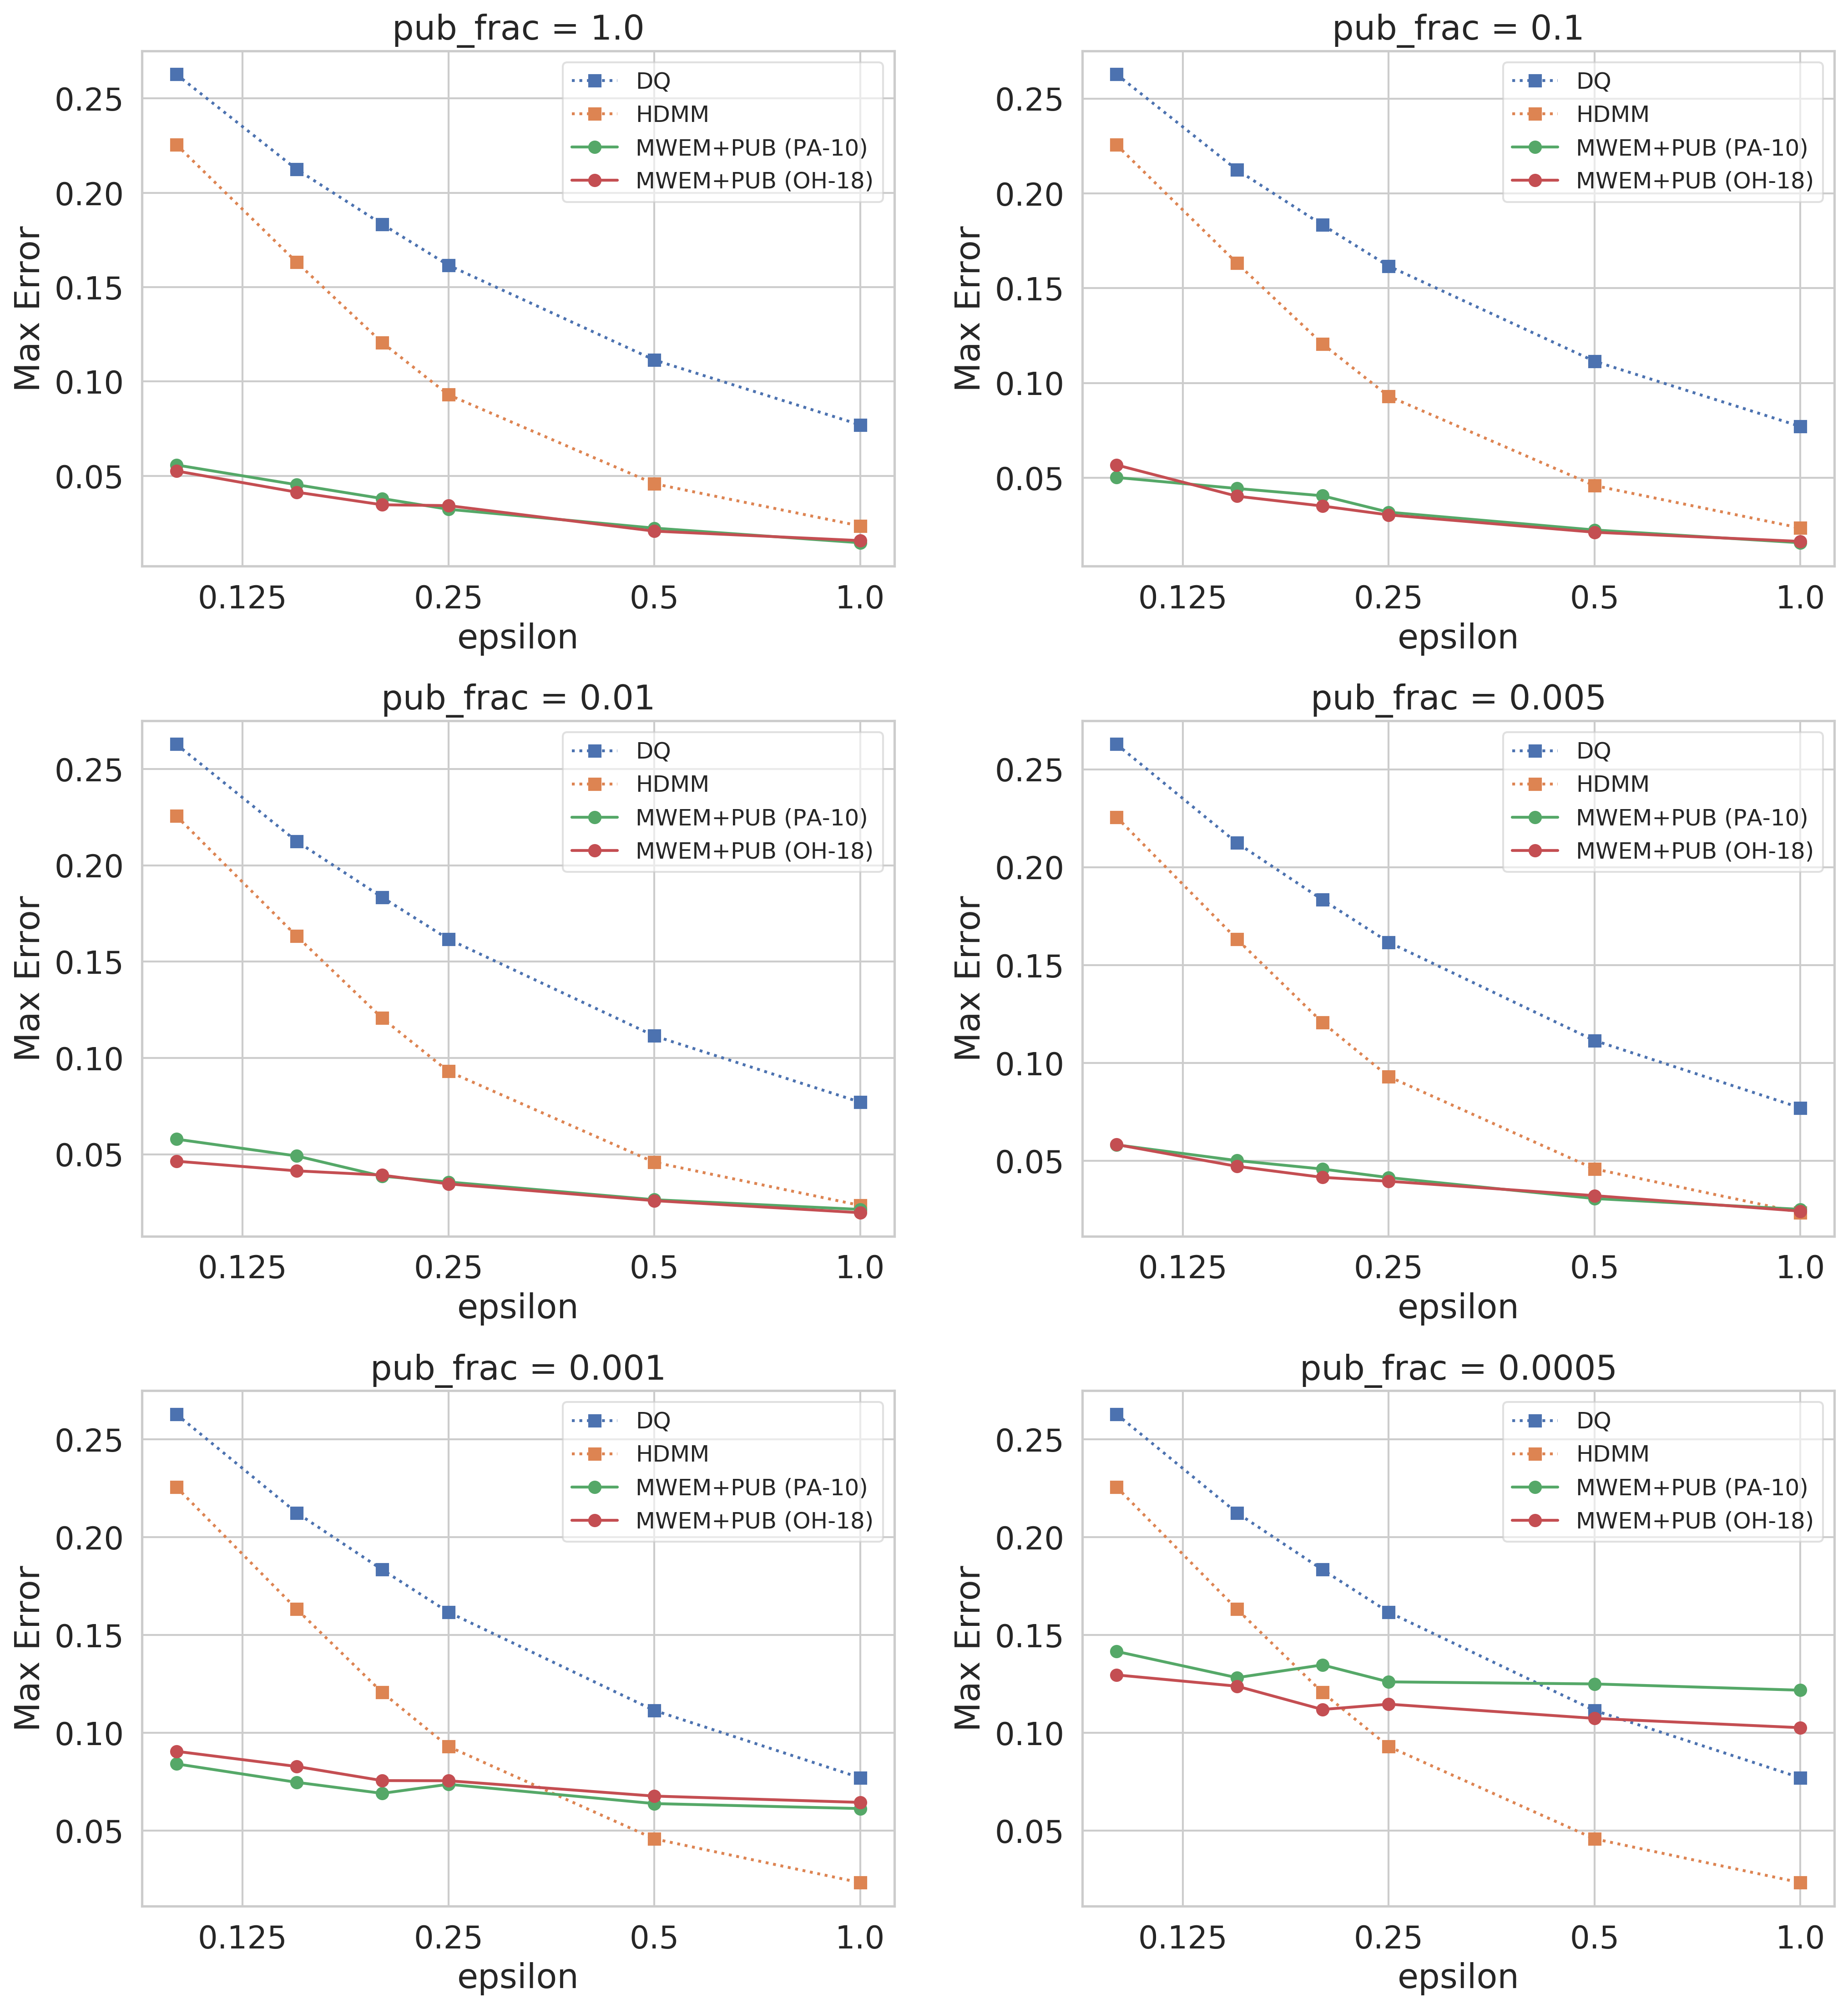}
    \caption{Max error on 3-way marginals across privacy budgets $\epsilon$ where $\delta = \frac{1}{N^2}$ and workload size is 4096. We vary the fraction of the public dataset used in each plot shown.}
    \label{fig:acs-pa_compare_benchmarks_appendix}%
\end{figure}
