# Supplementary material for: Leveraging Public Data for Practical Private Query Release
Source: arXiv:2102.08598 source file (2021-06-11)
Supplement: Supplementary file 2 [file compare_init.tex]

\begin{figure}[!htb]
    \centering
    \includegraphics[width=\linewidth]{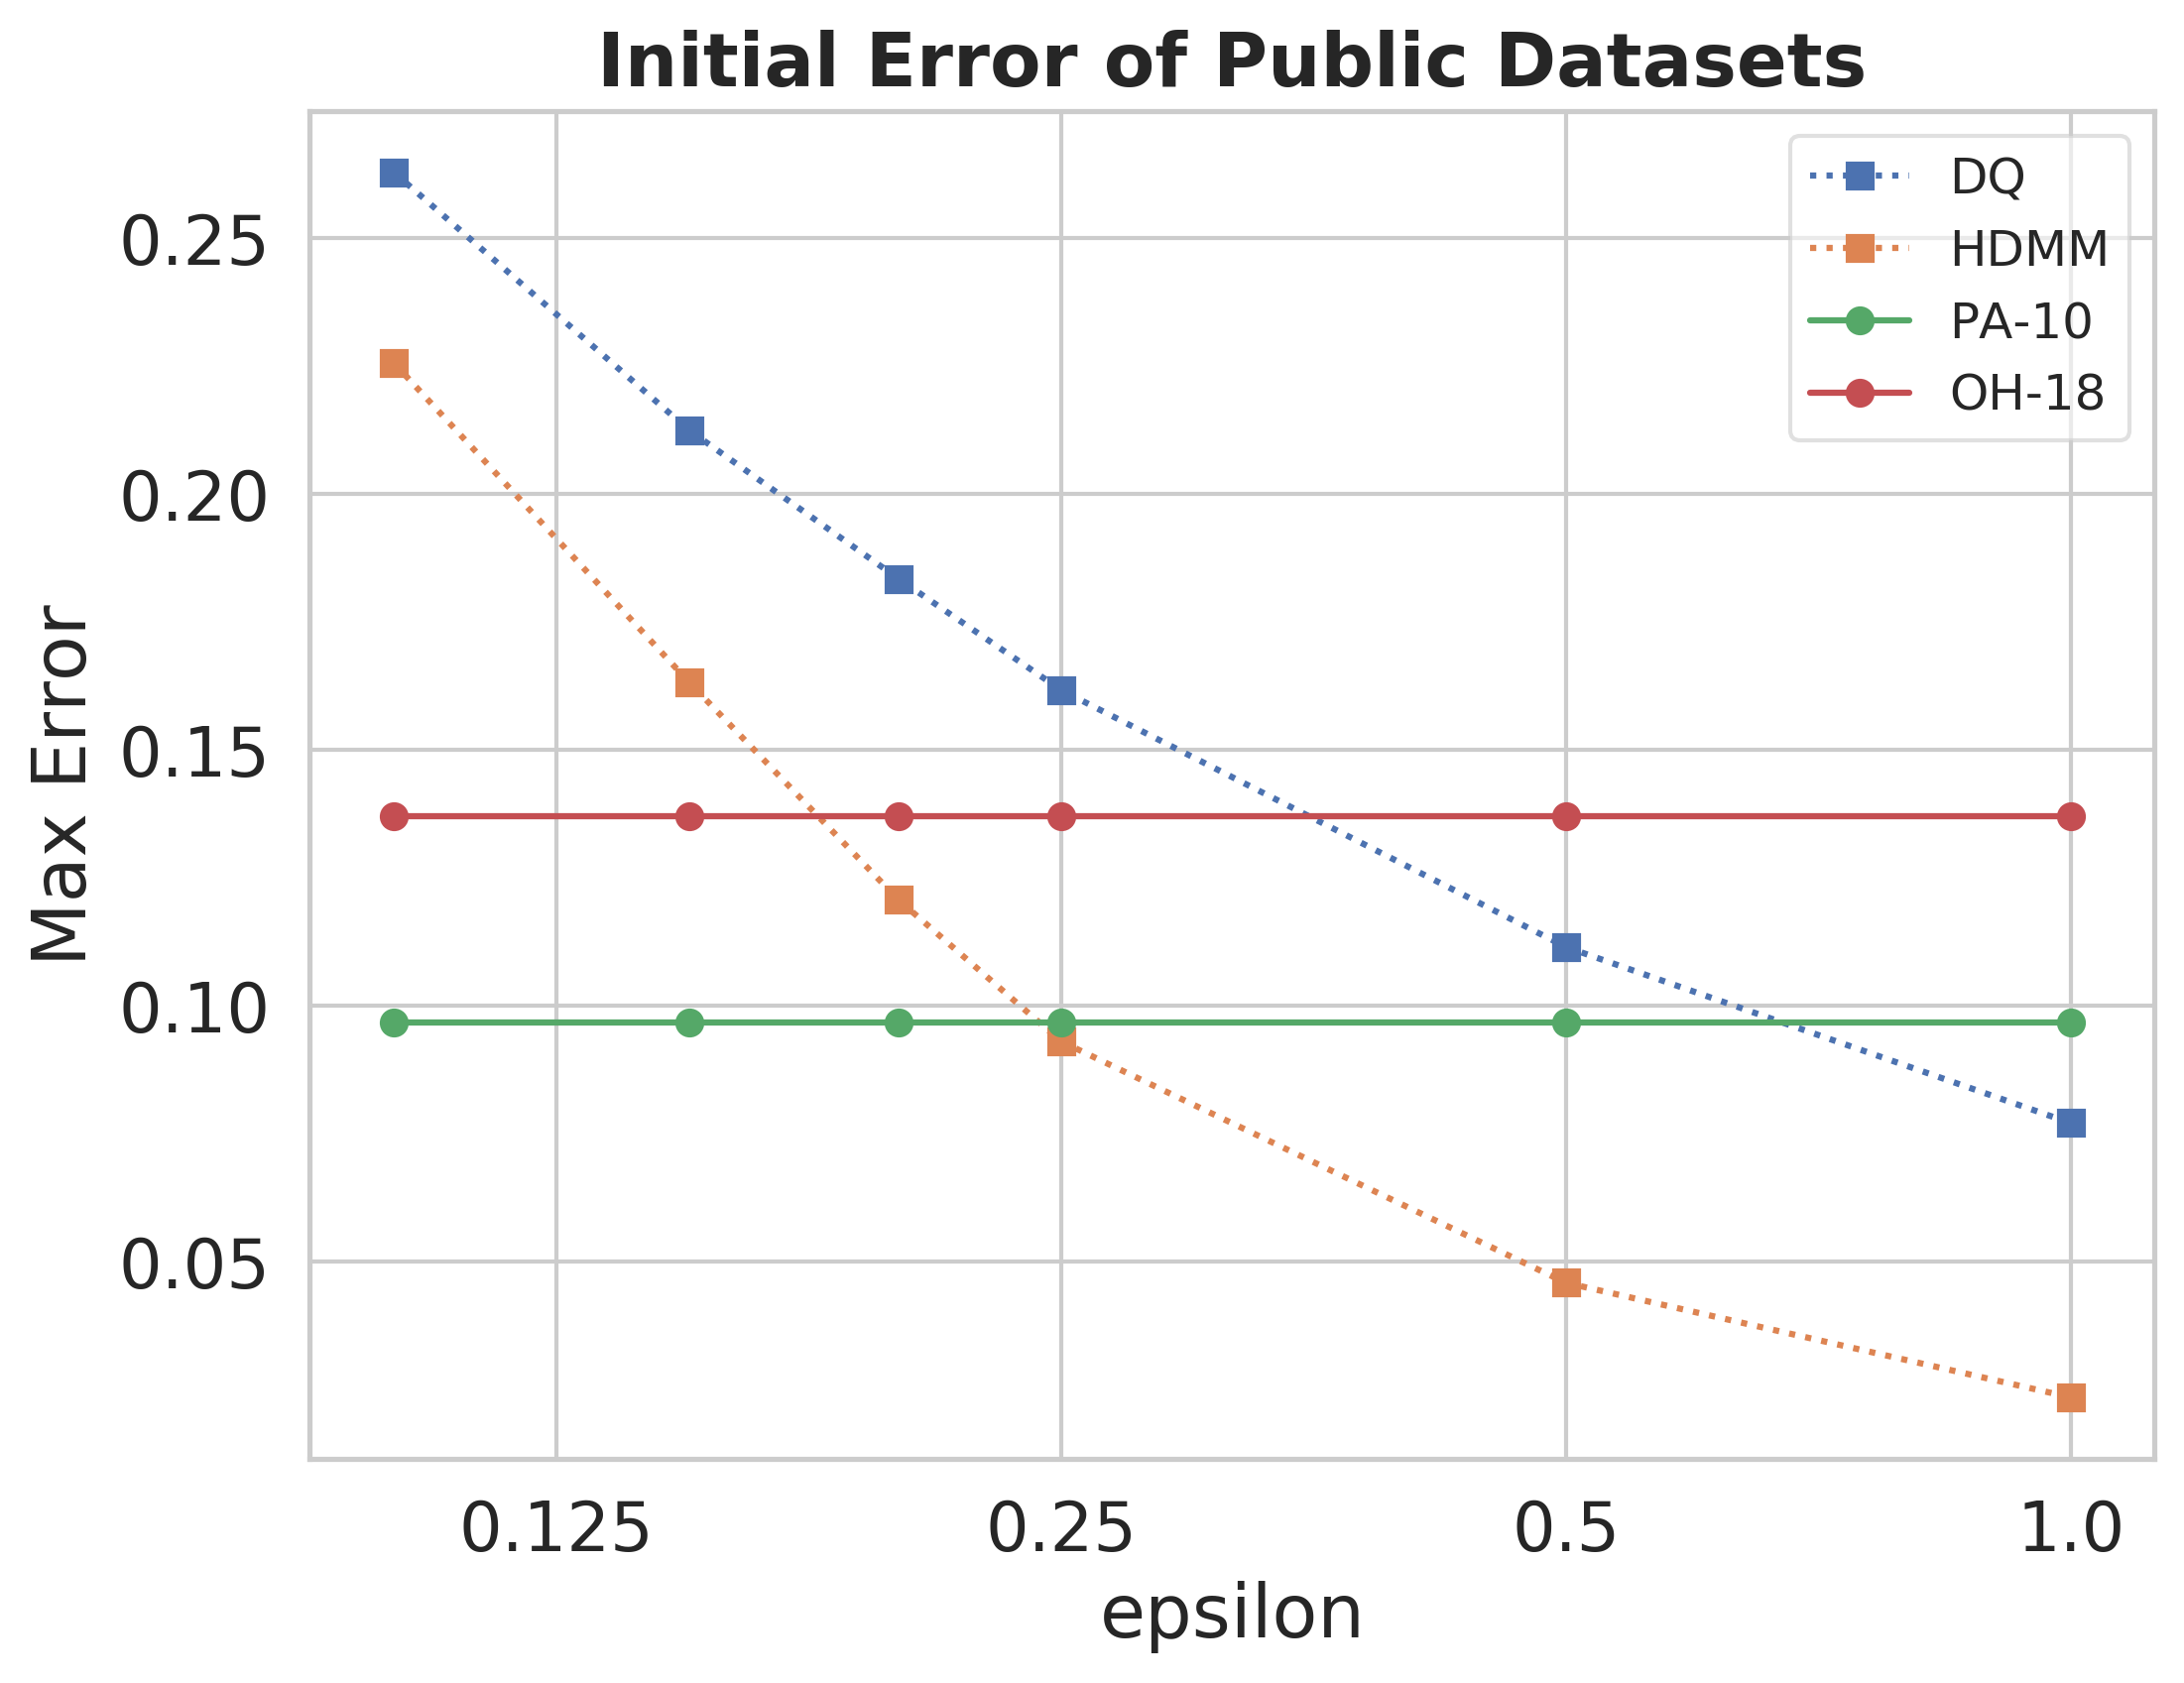}
    \caption{Max error on 3-way marginals across privacy budgets $\epsilon$ where $\delta = \frac{1}{N^2}$ and the workload size is 4096. \textbf{Bottom:} We evaluate the max error when using the public datasets to answer queries directly ($\epsilon = 0$).
    }
    \label{fig:acs-pa_compare_benchmarks}
\end{figure}
