# Supplementary material for: Leveraging Public Data for Practical Private Query Release
Source: arXiv:2102.08598 source file (2021-06-11)
Supplement: Supplementary file 3 [file compare_pub_sizes.tex]

\begin{figure}%
    \centering
    \includegraphics[width=\linewidth]{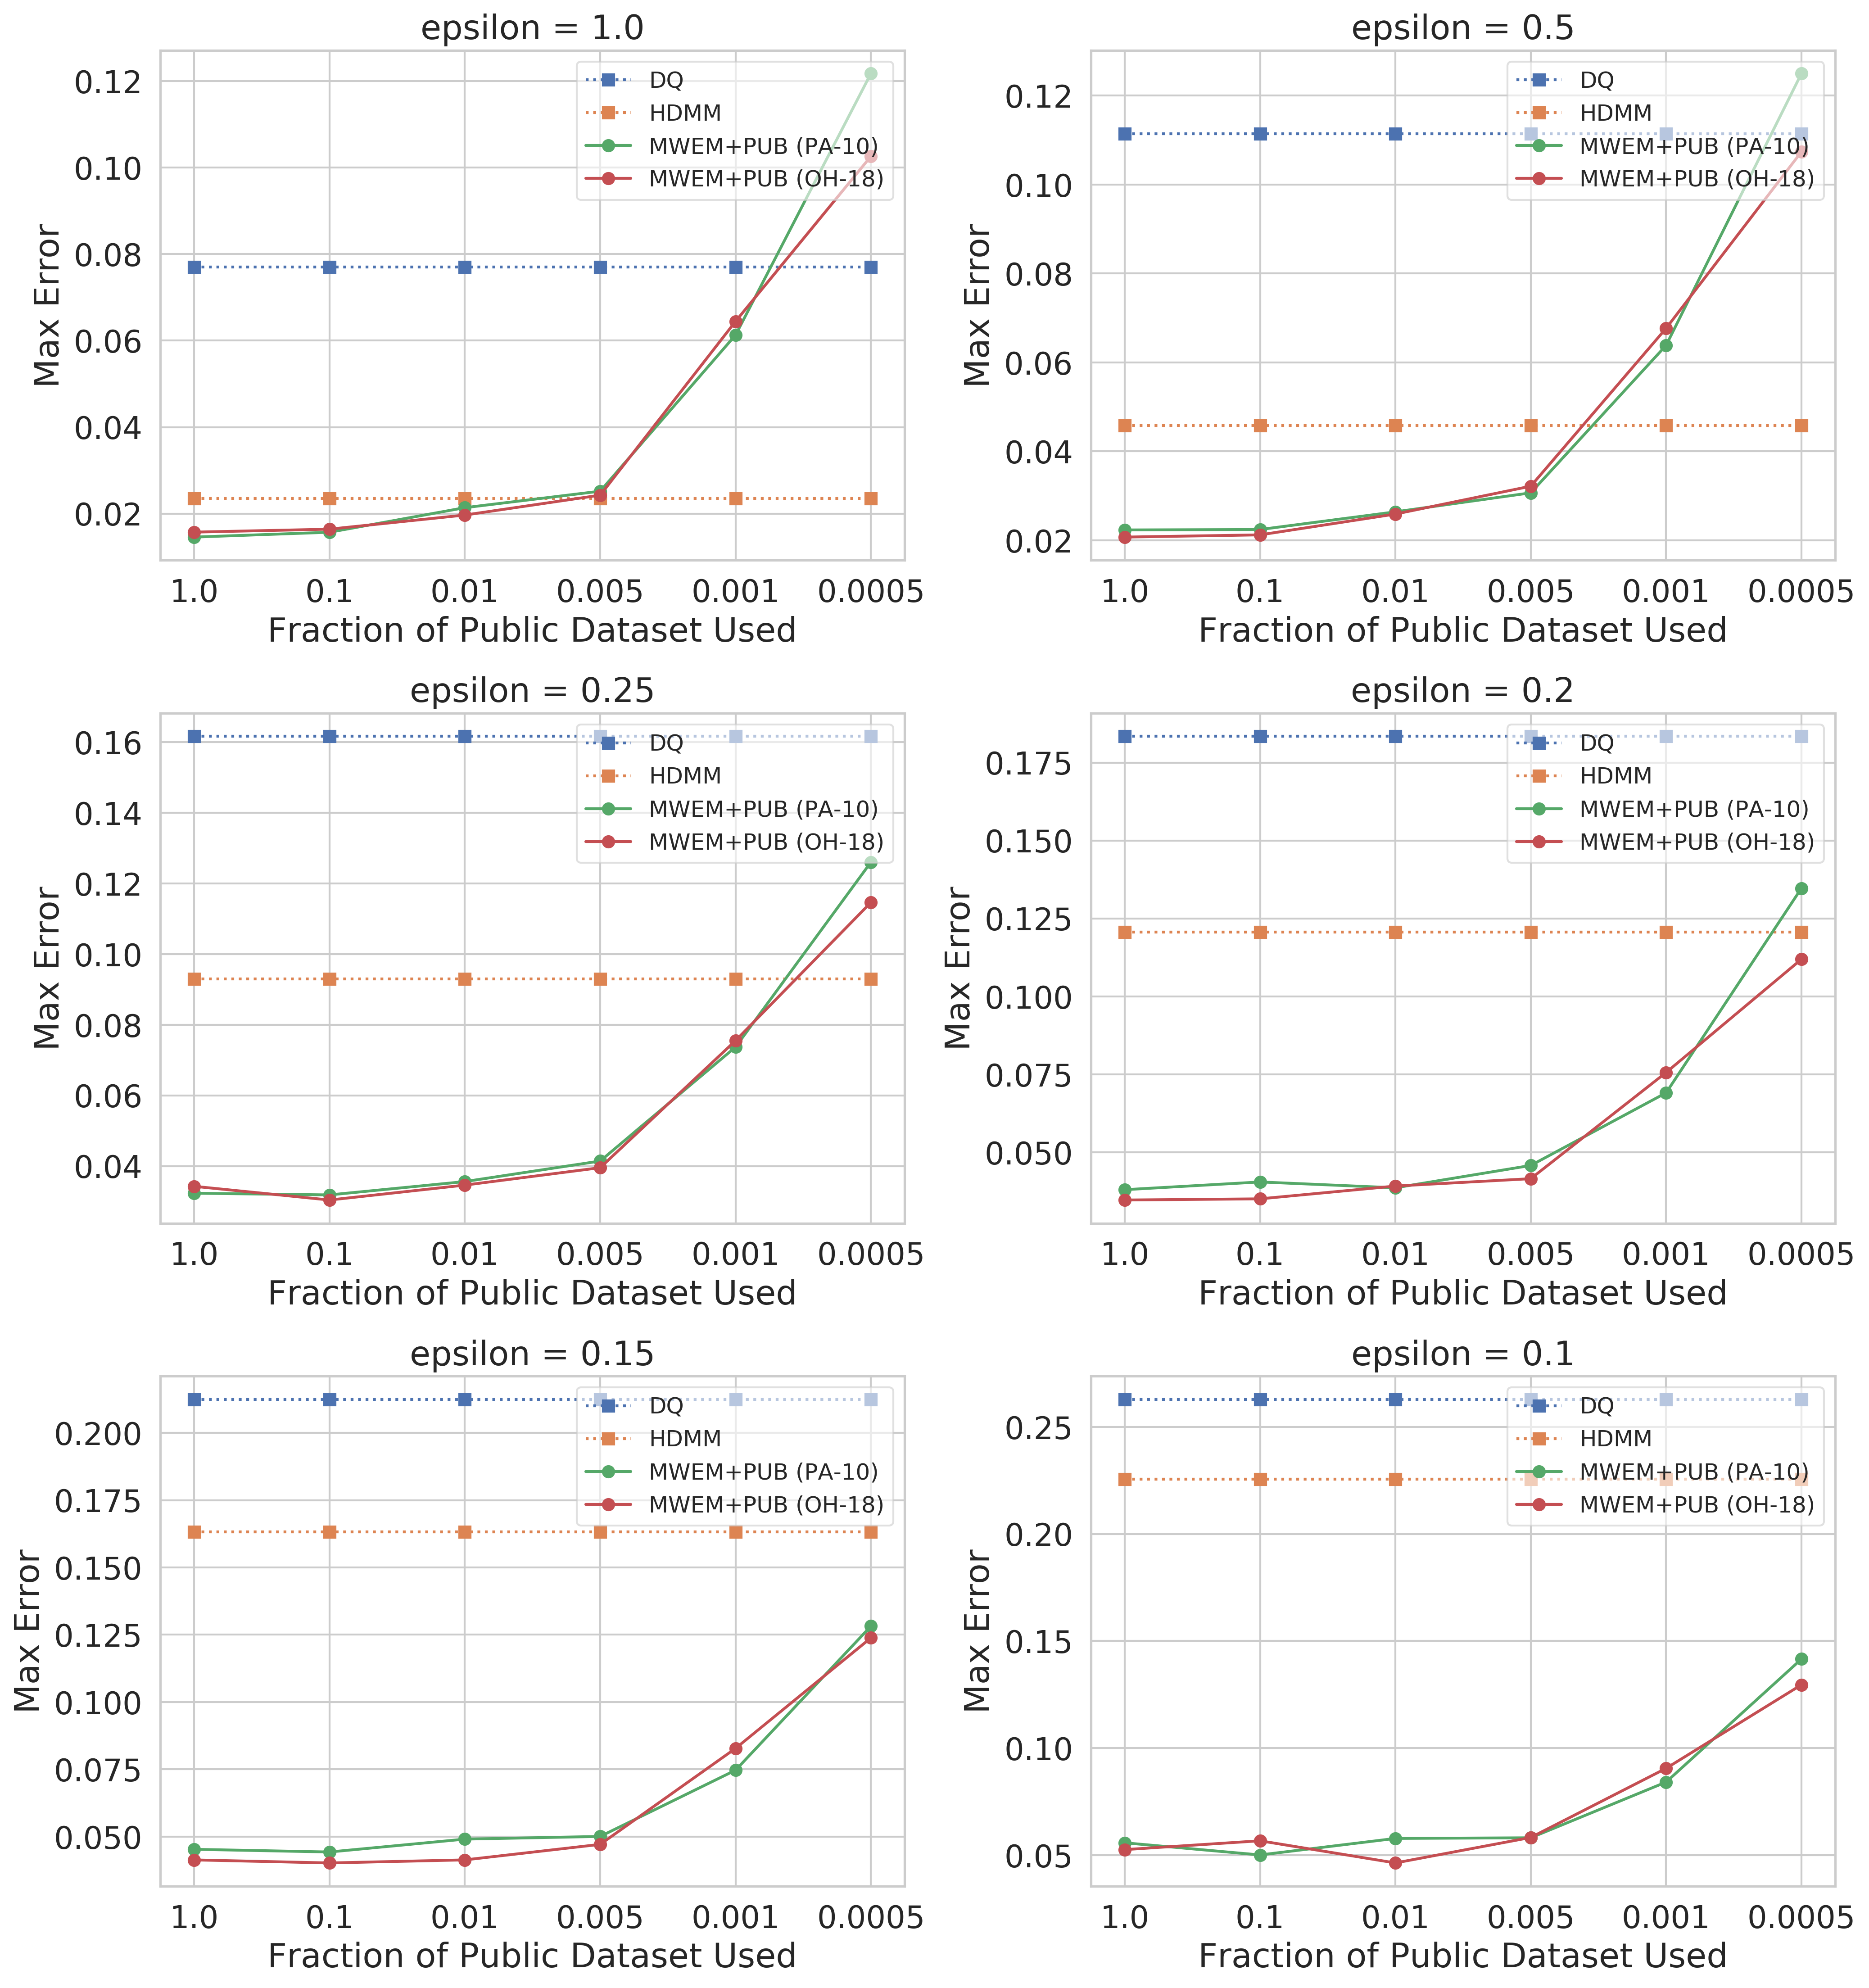}
    \caption{Comparison \ours to the benchmark algorithms on 3-way marginals with workload size as 4096 while varying the fraction of the public dataset used. We fix $\delta = \frac{1}{N^2}$ and vary $\epsilon$ for each plot shown.}
    \label{fig:acs-pa_compare_pub_sizes_appendix}%
\end{figure}
