# Supplementary material for: Leveraging Public Data for Practical Private Query Release
Source: arXiv:2102.08598 source file (2021-06-11)
Supplement: Supplementary file 4 [file compare_workloads_appendix.tex]

\begin{figure}%
    \centering
    \includegraphics[width=\linewidth]{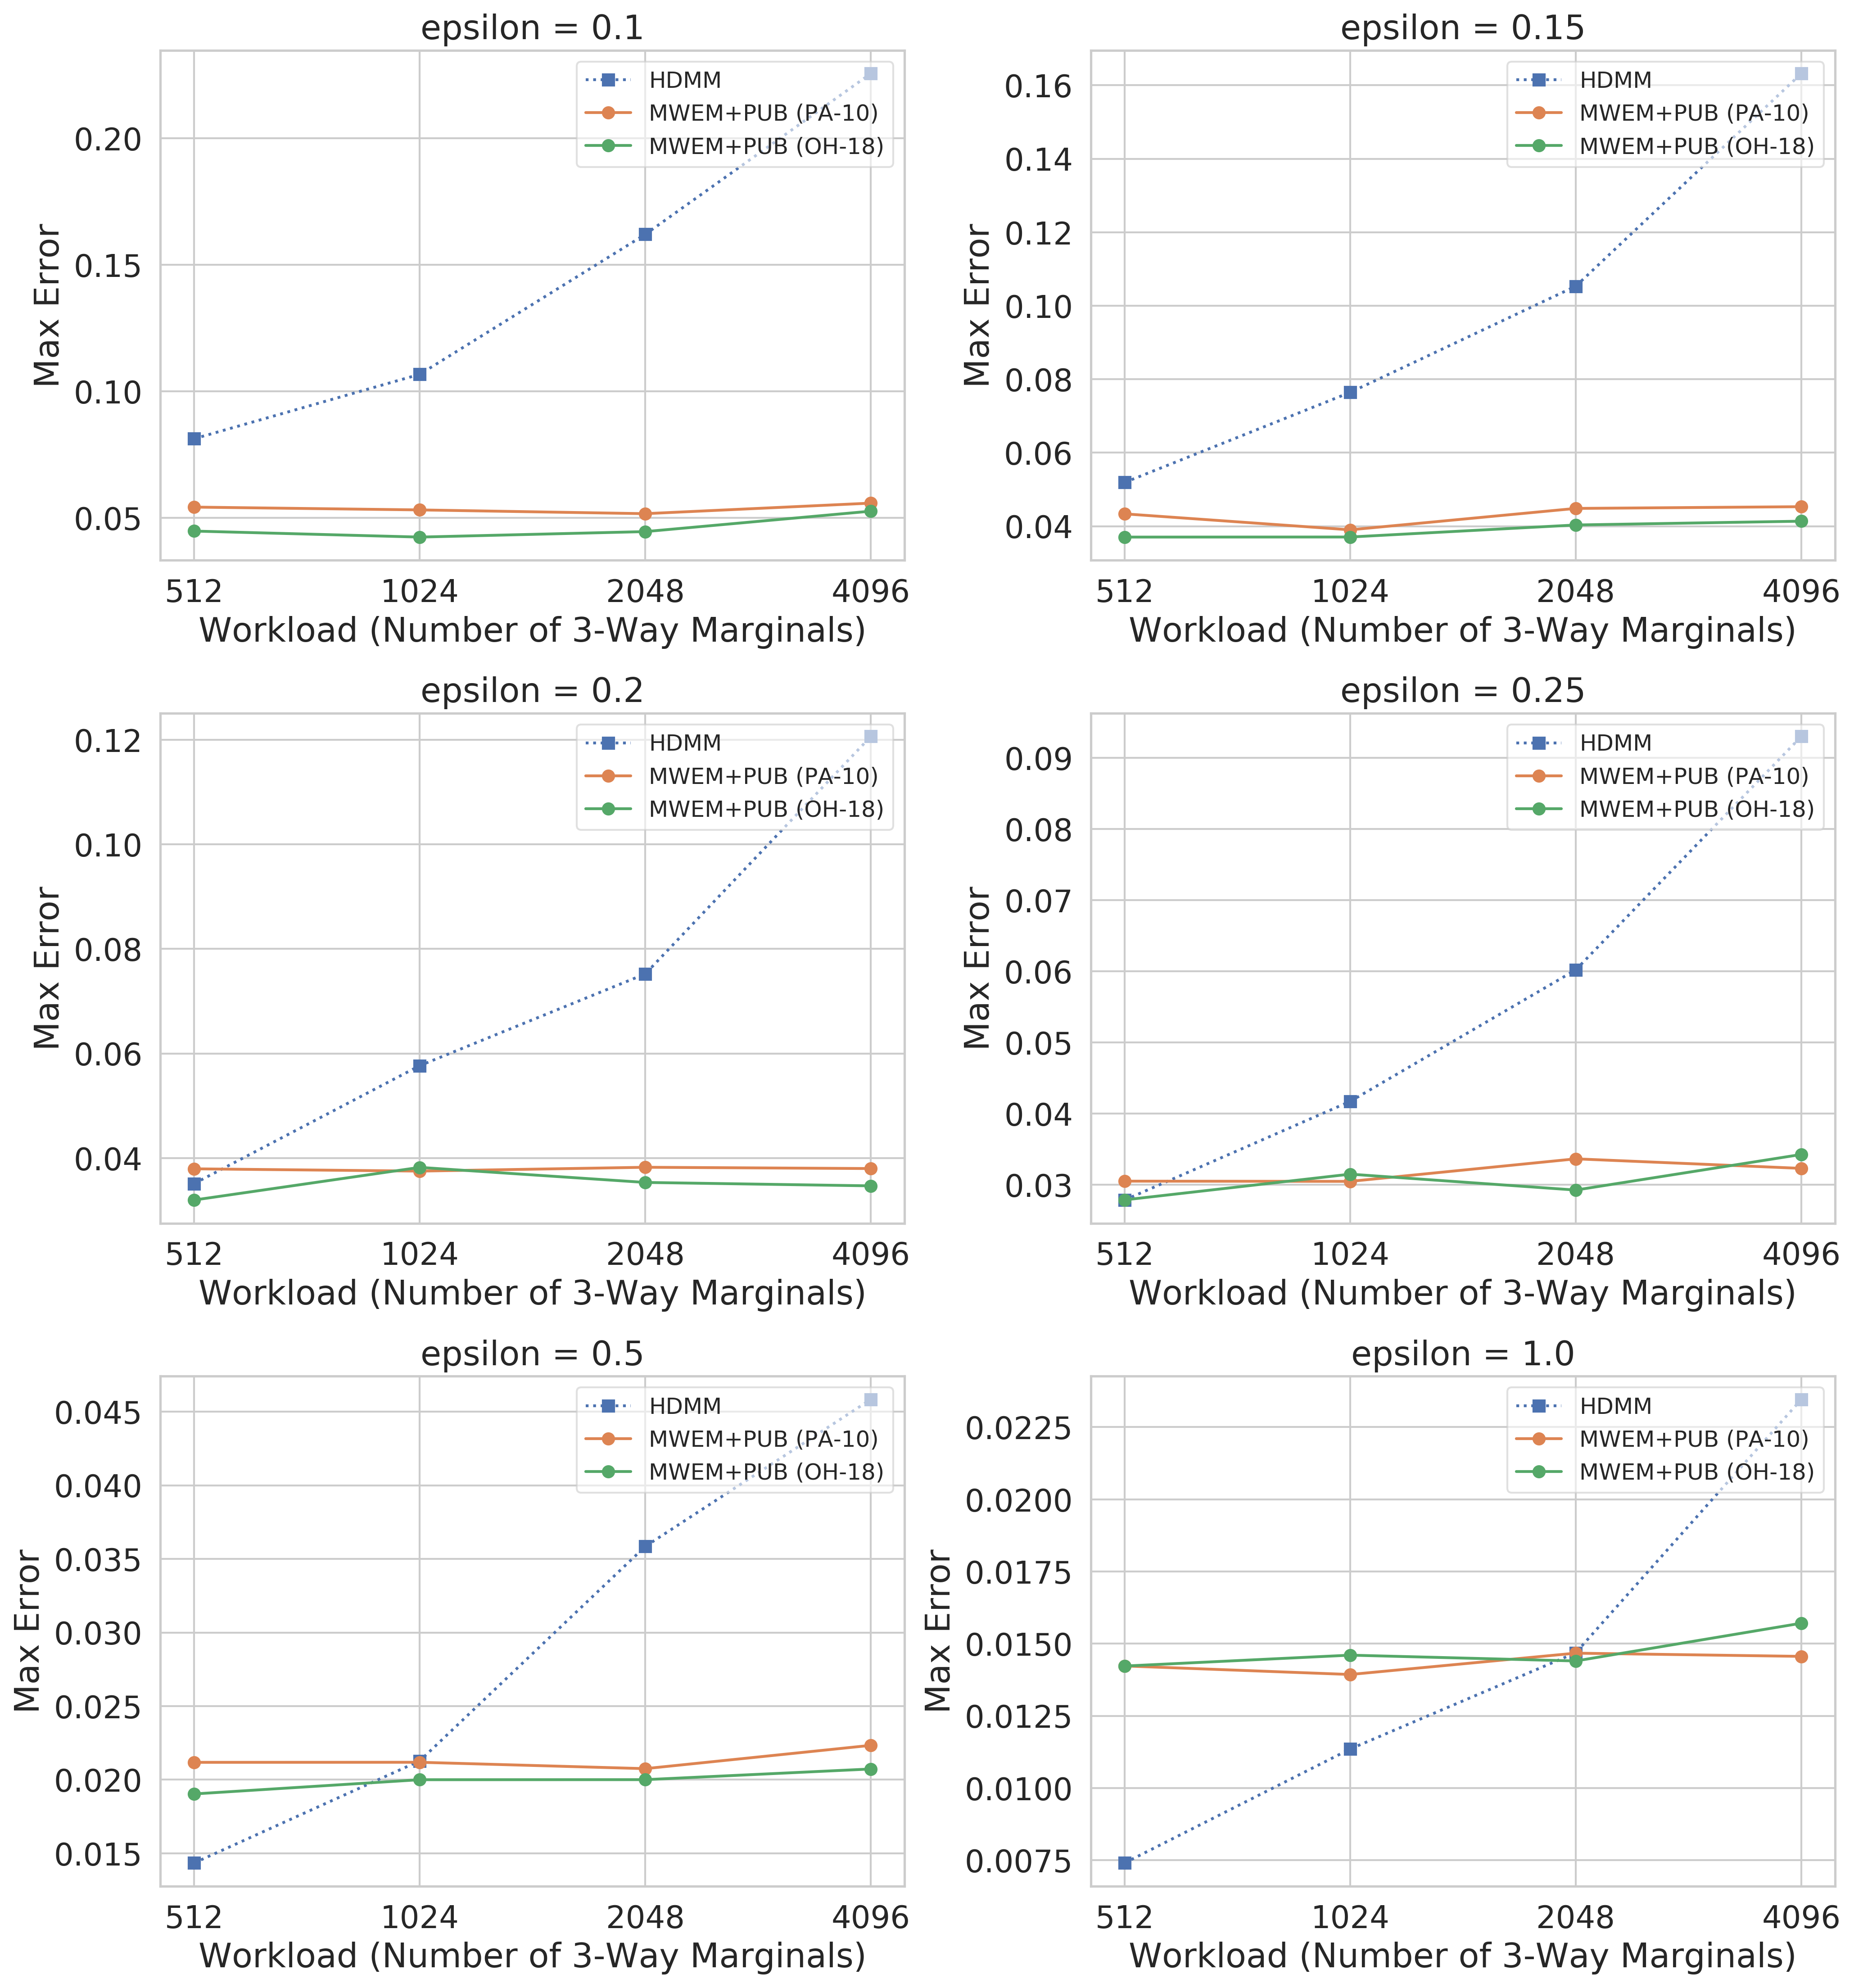}
    \caption{Comparison \ours (using the entire public dataset) against to HDMM on 3-way marginals while varying the workload size. We fix $\delta = \frac{1}{N^2}$ and vary the privacy budget $\epsilon$ in each plot shown.}
    \label{fig:acs-pa_compare_workloads_appendix}%
\end{figure}
