# Supplementary material for: Leveraging Public Data for Practical Private Query Release
Source: arXiv:2102.08598 source file (2021-06-11)
Supplement: Supplementary file 5 [file data_attributes.tex]

\begin{table*}
\begin{tabular}{l | c}
Parameter & Value \\
\textbf{ACS}
& ACREHOUS, AGE, AVAILBLE, CITIZEN, CLASSWKR, DIFFCARE, DIFFEYE, DIFFHEAR, \\
& DIFFMOB, DIFFPHYS, DIFFREM, DIFFSENS, DIVINYR, EDUC, EMPSTAT, FERTYR, \\ 
& FOODSTMP, GRADEATT, HCOVANY, HCOVPRIV, HINSCAID, HINSCARE, HINSVA, \\
& HISPAN, LABFORCE, LOOKING, MARRINYR, MARRNO, MARST, METRO, MIGRATE1, \\ 
& MIGTYPE1, MORTGAGE, MULTGEN, NCHILD, NCHLT5, NCOUPLES, NFATHERS, \\
& NMOTHERS, NSIBS, OWNERSHP, RACAMIND, RACASIAN, RACBLK, RACE, RACOTHER, \\ 
& RACPACIS, RACWHT, RELATE, SCHLTYPE, SCHOOL, SEX, SPEAKENG, VACANCY, \\ 
& VEHICLES, VET01LTR, VET47X50, VET55X64, VET75X90, VET90X01, VETDISAB, \\
& VETKOREA, VETSTAT, VETVIETN, VETWWII, WIDINYR, WORKEDYR \\
\textbf{ACS-small}
& DIFFEYE, DIFFHEAR, EMPSTAT, FOODSTMP, HCOVPRIV, HINSCAID, HINSCARE, \\
& OWNERSHP, RACAMIND, RACASIAN, RACBLK, RACOTHER, RACPACIS, RACWHT, SEX
\caption{MLP parameter configuration (Apps).}`
\end{tabular}
\label{table:attr}
\end{table*}
